# Supplementary material for: Preparation of Nuclear Spin Singlet States using Spin-Lock Induced Crossing
Source: arXiv:1307.0832 ancillary file (2013-07-02)
Supplement: Supplementary file 1 [file SLIC_1_supp-06-25-13.pdf]

# Supplementary Information: Preparation of Nuclear Spin Singlet States using Spin-Lock Induced Crossing

Stephen J. DeVience[a], Ronald L. Walsworth[b,c], Matthew S. Rosen[c,d,e]

[a] Department of Chemistry and Chemical Biology, Harvard University, 12 Oxford St., Cambridge, MA 02138

[b] Harvard-Smithsonian Center for Astrophysics, 60 Garden St., Cambridge, MA 02138

[c] Center for Brain Science, Harvard University, 52 Oxford St., Cambridge, MA 02138, USA

[d] Department of Physics, Harvard University, 17 Oxford St., Cambridge, MA 02138

[e] Harvard Medical School, 25 Shattuck Street, Boston, MA 02115

[f] A. A. Martinos Center for Biomedical Imaging, 149 Thirteenth St., Charlestown, MA 02129

## S1. Definitions of Density Matrices for Simulation

$$
\begin{aligned}
&I_{1x} + I_{2x} = |T_+\rangle\langle T_0| + |T_0\rangle\langle T_+| + |T_-\rangle\langle T_0| + |T_0\rangle\langle T_-| \\
&I_{1y} - I_{2y} = i\left(|T_+\rangle\langle S_0| + |S_0\rangle\langle T_+| - |T_-\rangle\langle S_0| - |S_0\rangle\langle T_-|\right) \\
&I_{1z} - I_{2z} = i\left(|T_0\rangle\langle S_0| + |S_0\rangle\langle T_0|\right) \\
&S_0 = |S_0\rangle\langle S_0| \\
&T_0 = |T_0\rangle\langle T_0|.
\end{aligned}
$$

## S2. Density Matrix Analysis of SLIC

An analysis of a two-spin system during spin-locking explains the mechanism of singlet creation. Consider a system of two coupled spin-1/2 nuclei with resonance frequencies $\nu_1$ and $\nu_2$, and let $\Delta\nu = \nu_1 - \nu_2$. The two spins have a scalar coupling $J$, and we will assume dipolar couplings are eliminated due to fast reorientation of the molecule, as in liquids. The Hamiltonian for this system written in the singlet/triplet basis is described by

$$\mathcal{H}_0 = h \begin{bmatrix} -\frac{\nu_1+\nu_2}{2} + \frac{J}{4} & 0 & 0 & 0 \\ 0 & \frac{J}{4} & 0 & \frac{\Delta\nu}{2} \\ 0 & 0 & \frac{\nu_1+\nu_2}{2} + \frac{J}{4} & 0 \\ 0 & \frac{\Delta\nu}{2} & 0 & -\frac{3J}{4} \end{bmatrix}, \tag{S1}$$

where the eigenstates are (from left to right) the three triplet states, $|T_-\rangle$, $|T_0\rangle$, and $|T_+\rangle$, and one singlet state, $|S_0\rangle$. These can be represented as symmetric and antisymmetric combinations of the product states:

$$\begin{aligned} |T_-\rangle &= |\uparrow\uparrow\rangle \\ |T_0\rangle &= \frac{|\uparrow\downarrow\rangle + |\downarrow\uparrow\rangle}{\sqrt{2}} \\ |T_+\rangle &= |\downarrow\downarrow\rangle \\ |S_0\rangle &= \frac{|\uparrow\downarrow\rangle - |\downarrow\uparrow\rangle}{\sqrt{2}}. \end{aligned} \tag{S2}$$

It is convenient to work in the rotating frame at the average resonance frequency of the nuclei, so that $(\nu_1+\nu_2)/2 = 0$. Then

$$\mathcal{H}_0 = h \begin{bmatrix} \frac{J}{4} & 0 & 0 & 0 \\ 0 & \frac{J}{4} & 0 & \frac{\Delta\nu}{2} \\ 0 & 0 & \frac{J}{4} & 0 \\ 0 & \frac{\Delta\nu}{2} & 0 & -\frac{3J}{4} \end{bmatrix}. \tag{S3}$$

If spin-locking is now applied on resonance with the triplet transitions with a nutation frequency $\nu_n$, the off-diagonal elements are added to the Hamiltonian to produce

$$\mathcal{H}_{SL} = h \begin{bmatrix} \frac{J}{4} & \frac{\nu_n}{\sqrt{2}} & 0 & 0 \\ \frac{\nu_n}{\sqrt{2}} & \frac{J}{4} & \frac{\nu_n}{\sqrt{2}} & \frac{\Delta\nu}{2} \\ 0 & \frac{\nu_n}{\sqrt{2}} & \frac{J}{4} & 0 \\ 0 & \frac{\Delta\nu}{2} & 0 & -\frac{3J}{4} \end{bmatrix}. \tag{S4}$$

Since the spin-locking is on for a long time relative to a precession period, it is best to rediagonalize the triplet states and study the resulting dressed states. The new dressed-state Hamiltonian is

$$\mathcal{H}_{SL,dressed} = h \begin{bmatrix} \frac{J}{4} - \nu_n & 0 & 0 & \frac{\Delta\nu}{2\sqrt{2}} \\ 0 & \frac{J}{4} & 0 & 0 \\ 0 & 0 & \frac{J}{4} + \nu_n & -\frac{\Delta\nu}{2\sqrt{2}} \\ \frac{\Delta\nu}{2\sqrt{2}} & 0 & -\frac{\Delta\nu}{2\sqrt{2}} & -\frac{3J}{4} \end{bmatrix}. \tag{S5}$$

and the resulting dressed states are

$$\begin{aligned} |\phi_-\rangle &= \frac{1}{2}(|\uparrow\uparrow\rangle + |\downarrow\downarrow\rangle - |\uparrow\downarrow\rangle - |\downarrow\uparrow\rangle) \\ &= \frac{1}{2}(|T_-\rangle + |T_+\rangle) - \frac{1}{\sqrt{2}}|T_0\rangle \\ |\phi_0\rangle &= \frac{1}{\sqrt{2}}(|\downarrow\downarrow\rangle - |\uparrow\uparrow\rangle) = \frac{1}{\sqrt{2}}(|T_+\rangle - |T_-\rangle) \\ |\phi_+\rangle &= \frac{1}{2}(|\uparrow\uparrow\rangle + |\downarrow\downarrow\rangle + |\uparrow\downarrow\rangle + |\downarrow\uparrow\rangle) \\ &= \frac{1}{2}(|T_-\rangle + |T_+\rangle) + \frac{1}{\sqrt{2}}|T_0\rangle \\ |\phi_S\rangle &= \frac{1}{\sqrt{2}}(|\uparrow\downarrow\rangle - |\downarrow\uparrow\rangle) = |S_0\rangle. \end{aligned} \tag{S6}$$

The states $|\phi_0\rangle$ and $|\phi_S\rangle$ are split by energy $J$ and are unaffected by the strength of spin-locking, whereas the energies of states $|\phi_-\rangle$ and $|\phi_+\rangle$ have a linear dependence on $\nu_n$.

It is now evident that selecting a nutation frequency $\nu_n = J$ will match the energies of states $|\phi_-\rangle$ and $|\phi_S\rangle$, creating a spin-lock induced crossing. At this energy, the off-diagonal interaction terms $\Delta\nu/2\sqrt{2}$ become significant and promote polarization transfer. These cause polarization to oscillate between triplet and singlet states with a period of $\sqrt{2}/\Delta\nu$, and maximimum transfer occurs at half this time:

$$t_{SL,max} = \frac{1}{\Delta\nu\sqrt{2}} = \frac{0.707}{\Delta\nu}. \tag{S7}$$

## S3. Further Experimental Details

Measurements were performed on a 20 mM solution of the tripeptide phenylalanine-glycine-glycine (phe-gly-gly, Sigma Aldrich) prepared in $D_2O$. Nitrogen gas was bubbled through the solution for 5 minutes to displace dissolved oxygen. Proton NMR spectra were acquired with a Bruker 4.7 T spectrometer at 200 MHz. A reference spectrum was acquired with one 90 degree pulse followed by an FID (free-induction decay) acquisition. The spin-lattice relaxation time, $T_1$, was measured for each nucleus using an inversion recovery sequence.

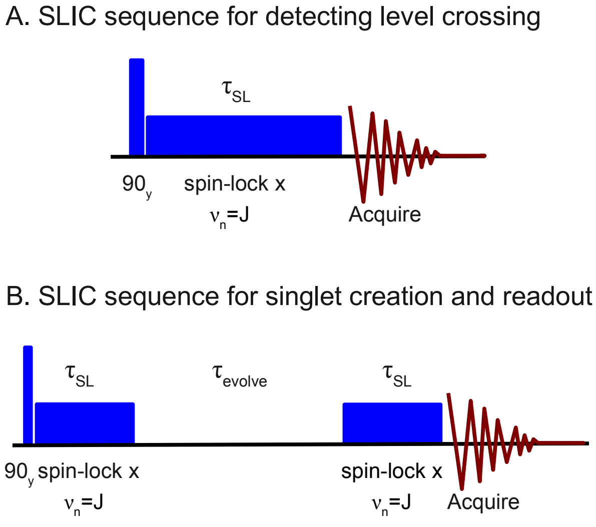


Figure S1: A typical experiment uses the SLIC sequence to create singlet by applying spin-locking with the nutation frequency matched to the J-coupling for a duration appropriate for the resonance frequency difference. (A) The acquisition can be performed directly following singlet creation to detect the corresponding drop in x-axis magnetization, or (B) the system can be allowed to evolve, and singlet can be converted back to transverse polarization for readout by applying spin-locking a second time.

Pulse sequences to implement SLIC are shown in Fig. S1. The transmitter frequency is set to the average resonance frequency of the proton pair of interest. A $\pi/2$ pulse is applied to create a coherence between $(|T_-\rangle + |T_+\rangle)\sqrt{2}$ and $|T_0\rangle$. Next, the phase is shifted 90 degrees and spin-locking is applied with a nutation frequency $\nu_n = J$. In the resulting dressed state, the previous coherence becomes a population difference between $|\phi_-\rangle\langle\phi_-|$ and $|\phi_+\rangle\langle\phi_+|$. After a time $\tau_{SL} = 0.707/\Delta\nu$, this is converted to a population difference between $|\phi_S\rangle\langle\phi_S|$ and $|\phi_+\rangle\langle\phi_+|$. Spin-locking is then removed. In Fig. S1A, an acquisition is performed immediately to measure the x-axis magnetization, $I_{1x} + I_{2x}$, whereas in Fig. S1B the system is allowed to evolve for duration $\tau_{evolve}$ and both the singlet and triplet states are allowed to relax. The remaining singlet polarization is then read out by applying spin-locking again at 90 degrees phase with power $\nu_n = J$ for time $\tau_{SL}$ and then acquiring an FID at phase 0 degrees. Phase cycling is performed to remove residual triplet polarization by inverting the phase of the $\pi/2$ pulse and the acquisition. The singlet state lifetime is found by measuring the remaining singlet population for a range of $\tau_{evolve}$ and fitting to a single exponential decay.

For comparison, we also performed the experiment using Levitt's M2S sequence for preparation and readout of the singlet state, with the pulse sequence drawn in Fig. 1A of the main text. The single delay time used in the M2S sequence is set to $\tau = 1/4J$, and the number of cycles for the first and second pulse trains are $n_1 = \pi/2\theta$ and $n_2 = \pi/4\theta$, where $\theta$ is the rotation out of the singlet-triplet basis caused by the resonance frequency difference. This rotation depends on the ratio of $\Delta\nu$ to $J$ and is given by

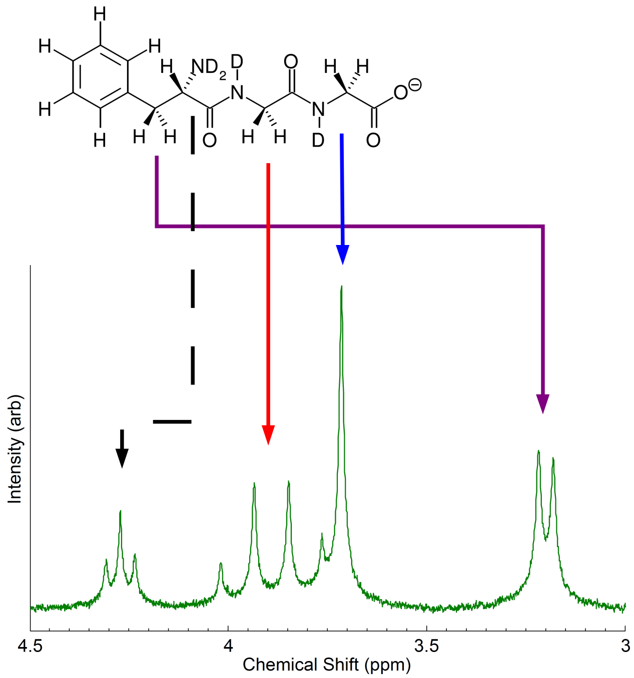


Figure S2: The phenylalanine-glycine-glycine structure is shown with its corresponding spectrum at 200 MHz. The aromatic proton resonances occurs near 7.3 ppm and are not shown. Line broadening of 0.1 Hz was applied.

$$\theta = \tan^{-1}\frac{\Delta\nu}{J}. \tag{S8}$$

The optimal number of pulses can vary significantly from the theoretical values when other spins couple to the target spin pair.

We optimized the singlet state creation for SLIC using both sequences of Fig. S1 by scanning $\nu_n$ and $\tau_{SL}$ and measuring the NMR signal at the end of each sequence. For the M2S sequence, we optimized parameters by scanning $\tau$, $n_1$, and $n_2$ and measuring the NMR signal at the end of the sequence.

## S4. Spectrum of Phenylalanine-Glycine-Glycine

The proton NMR spectrum of phenylalanine-glycine-glycine (Fig. S2) reveals that the molecule possesses two sets of nearly-equivalent proton pairs ($\delta = 3.20$ ppm and $\delta = 3.71$), and one proton pair exhibiting a second-order spectrum (centered at $\delta = 3.89$ ppm). Each proton of the $\delta = 3.20$ ppm pair is split by a third neighboring spin ($\delta = 4.27$ ppm) with strength $J = 7.3$ Hz. Spin lattice relaxation times were measured and are summarized in Table 1.

Table S1: Spin-lattice relaxation times for the phe-gly-gly protons.

| Chemical Shift ($\delta$) | $T_1$ (ms) | | |
|---|---|---|---|
| 3.20 | 430 | $\pm$ | 5 |
| 3.71 | 912 | $\pm$ | 7 |
| 3.89 | 618 | $\pm$ | 6 |
| 4.27 | 1760 | $\pm$ | 20 |

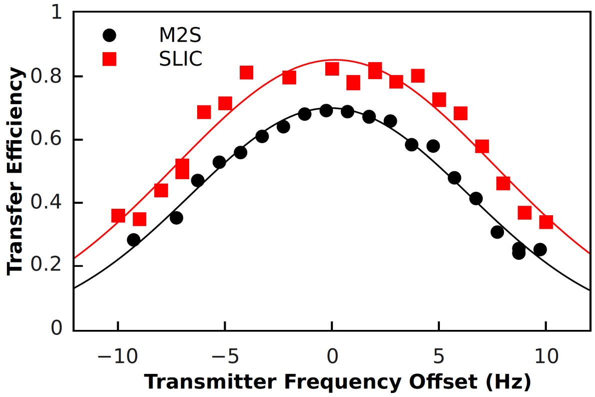


Figure S3: The triplet/singlet polarization transfer efficiencies for SLIC and M2S were measured as a function of transmitter frequency offset. SLIC had a higher efficiency and a slightly broader effective bandwidth.

## S5. Effective bandwidth of M2S and SLIC

We compared the effectiveness of M2S and SLIC using off-resonant transmitter frequencies. We performed singlet creation and readout sequences using both M2S and SLIC at a number of transmitter frequency offsets with a constant $\tau_{evolve} = 500$ ms and measured the transfer efficiency. The resulting curves were fit with a Gaussian to determine a full-width half max (FWHM) effective bandwidth (Fig. S3). The effective bandwidth was similar for both sequences, with FWHM bandwidths of 17.6 $\pm$ 0.6 Hz for SLIC and 15.3 $\pm$ 0.3 Hz for M2S.
